# Supplementary material for: VALHALLA: Visual Hallucination for Machine Translation
Source: arXiv:2206.00100 source file (2022-05-31)
Supplement: Supplementary file 2 [file optim.tex]

\begin{table*}[ht]
\centering
\caption{\textbf{Optimization Hyperparameters.}
\todo{Learning rate schedule, dropout, label smoothing, }}
\label{tab:optim}
\end{table*}
